# Supplementary material for: Multi-view 3D Reconstruction of a Texture-less Smooth Surface of Unknown Generic Reflectance
Source: arXiv:2105.11599 source file (2021-05-25)
Supplement: Supplementary file 1 [file supplementary.pdf]

# Supplementary Materials:

## Multi-view 3D Reconstruction of a Texture-less Smooth Surface of Unknown Generic Reflectance

Ziang Cheng<sup>1</sup>, Hongdong Li<sup>1</sup>, Yuta Asano<sup>2</sup>, Yinqiang Zheng<sup>3</sup>, Imari Sato<sup>2</sup>

<sup>1</sup>Australian National University

<sup>2</sup>National Institute of Informatics, <sup>3</sup>The University of Tokyo, Japan

{ziang.cheng, hongdong.li}@anu.edu.au

### 1. Learning BRDF bases from MERL dataset

This section provides further implementation details of how to learn the BRDF bases. Given a collection of real world log-BRDFs, the set of PCA bases  $\mathcal{D}$  can be found by finding  $N$  eigen-functions of the function space. Since our training set (*i.e.* MERL [3]) records only BRDF values at discretely sampled incident angles  $\theta$  (*i.e.*  $\theta \in \{0, 1, 2, \dots, 89\}$ ), we estimate the BRDF-value at any angle via interpolation. Formally, given a collection of sampled BRDFs stored as a matrix  $Q$  whose columns each represents a distinct BRDF, we define the  $i_{\text{th}}$  basis function of  $\mathcal{D}$  as

$$d_i = \text{interp}(u_i s_i), \quad \text{where } \log Q \stackrel{\text{svd}}{=} USV \quad (13)$$

where  $u_i$  is the  $i_{\text{th}}$  leading left singular vector of  $\log Q$ , and  $s_i$  the corresponding singular value. *interp* is an interpolation operator that returns a continuous function (log-BRDF bases) from its discrete sampling. We used linear interpolation. The mean BRDF  $\mu(\cdot)$  can be similarly interpolated from the row wise mean of  $\log Q$ . This interpolation gives rise to continuous basis functions, though with one caveat of losing exact orthogonality of the bases. However, in practice we found this effect can be safely ignored.

We also scale down ‘less prominent’ basis functions by weighing them using their corresponding singular values. As a result, the parameter  $\mathbf{c}$  follows a spherical distribution in training BRDF space, and  $E_c(\mathbf{c})$  becomes an isotropic penalty on  $\mathbf{c}$ . Note that, the regression of  $\mathbf{c}$  is inspired by the ridge regression [4, 5]. In [2] Hui *et al.* used a similar dictionary-based BRDF model with sparseness constrains by solving a LASSO regression. However, we found the generalization ability of their method is inferior compared with our model.

### 2. Additional Experiment Results

More experiment results are provide in this section to illustrate the performance of our method.

#### 2.0.1 BRDFs used for synthetic experiments

Table 1 lists the BRDFs used for the 5-round cross validation in our synthetic experiments. The 25 testing BRDFs cover a wide range of materials from diffusive (*e.g.* fabric/rubber/latex), mildly specular (*e.g.* plastics/quartz/marble), to highly specular (*e.g.* metals/metallic paints/crystals).

#### 2.0.2 Visualization of reconstructed shape from synthetic images

Fig. 1 illustrates examples of recovered point cloud.

As a bonus case, we include an open and smooth surface (Himmelblau’s function) as the 5<sub>th</sub> model in our synthetic experiments. The surface is boundless, smoothly varying and made from highly specular materials, which is extremely challenging for shape-from-silhouette and multi-view stereo methods. 10 views are rendered as inputs for reconstruction. Fig. 2 illustrates the shape and reconstruction results of Himmelblau’s function.

#### 2.0.3 Robustness to non-ideally co-located configuration or anisotropic light source.

While our algorithm assumes an isotropic point light source that is co-located with camera optical centre, this setup can become impractical for real-world applications. In fact, most commodity point light sources (*e.g.* LED bulbs) exhibit anisotropic radial intensity distribution (RID), and a beam-splitter is typically necessary to facilitate the co-localisation of light and camera. Additionally, the light

**Table 1:** Testing BRDFs in MERL dataset for each round of cross validation.

| round      | 1                                                                                       | 2                                                                                   | 3                                                                            | 4                                                                                        | 5                                                                              |
|------------|-----------------------------------------------------------------------------------------|-------------------------------------------------------------------------------------|------------------------------------------------------------------------------|------------------------------------------------------------------------------------------|--------------------------------------------------------------------------------|
| test BRDFs | alumina-oxide<br>black-obsidian<br>black-phenolic<br>black-soft-plastic<br>white-marble | gray-plastic<br>pink-jasper<br>chrome<br>silicon-nitride<br>specular-black-phenolic | ss440<br>tungsten-carbide<br>white-acrylic<br>red-specular-plastic<br>delrin | color-changing-paint1<br>gold-metallic-paint<br>red-fabric<br>green-latex<br>pure-rubber | steel<br>alum-bronze<br>red-metallic-paint<br>chrome-steel<br>tungsten-carbide |

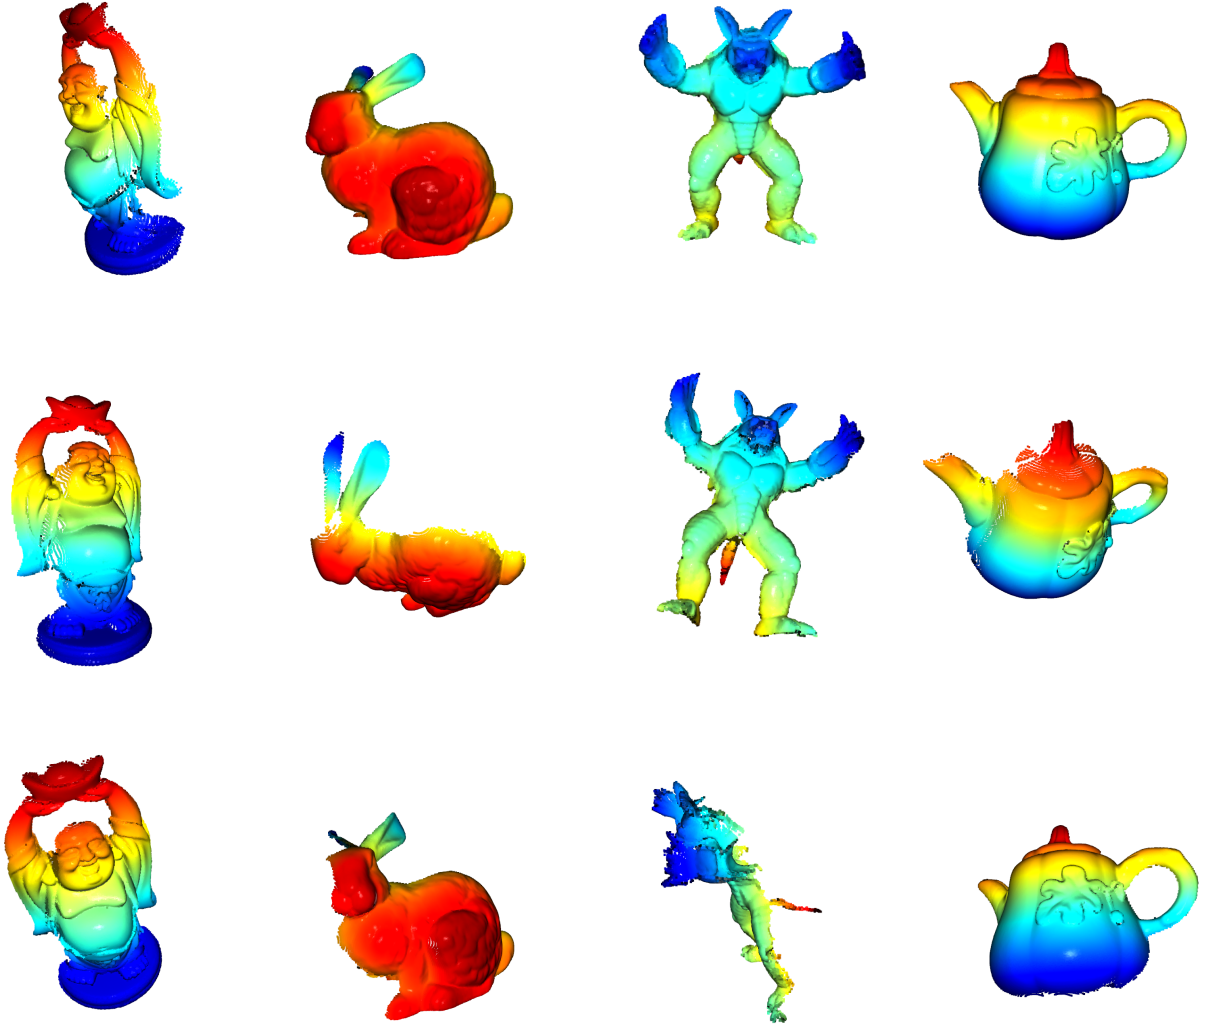

**Figure 1:** Recovered point cloud rendered from novel viewpoints.

source would need to be calibrated before use. Notwithstanding, we found that the algorithm is reasonably robust to slightly misplaced or anisotropic light even without calibration.

- Fig. 3a illustrates how performance degrades as dis-

placement increases, where the displacement is always in camera's x-axis and is measured in world units.<sup>1</sup>

An interesting observation is the performance does not

<sup>1</sup>We vary displacement from zero to the target object's span, *i.e.* 0.25 world unit or 25 centimetres.

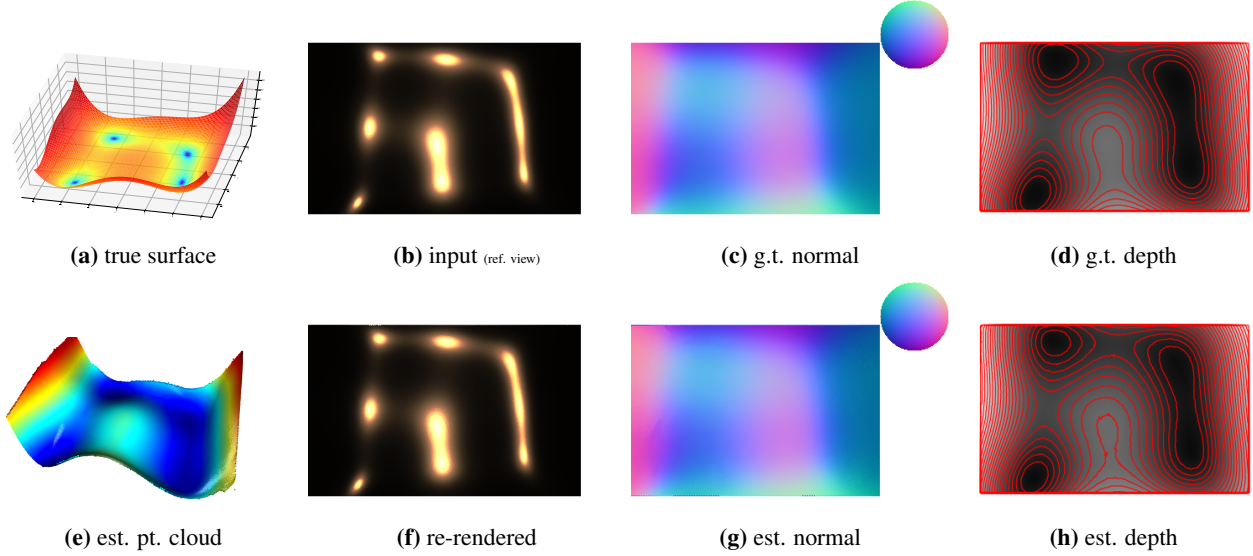

**Figure 2:** Reconstruction of a boundless, smooth surface (bird's-eye view of Himmelblau's function); contours are overlaid on the depth map from which we can see four global minima.

start to deteriorate - but rather marginally improves in depth and BRDF estimation - with a small displacement. Perhaps uncoincidentally, such displacement also leads to a small optimal difference angle for minimal BRDF sampling [4].

- Fig. 3b shows how performance degrades with an anisotropic RID modeled by  $\cos^\phi(\theta)$ , where  $\theta$  is the angle between out-going light ray and principal axis of light source<sup>2</sup> and  $\phi$  controls the anisotropy of RID ( $\phi = 0$  yields isotropic light source) as illustrated in Fig. 3c. It is seen that the setup is robust to even strongly anisotropic light source, which is expected since the target's angular extent in each view is limited (apprx. 20 degrees).

#### 2.0.4 More real image tests.

Fig. 4 shows the input reference image, recovered shape and re-rendered image with recovered reflectance.

### 3. Finding the globally optimal solutions of $\{\mathbf{n}, \mathbf{z}\}$ in Eq. (12).

Here we show Eq. (12) can be globally minimized over  $\{\mathbf{n}, \mathbf{z}\}$  direction. We start by dissecting this optimization

<sup>2</sup>Here we assume light source and camera are co-axial when rendering images.

into the summation of  $|K|$  independent sub-problems, *i.e.*

$$\min_{\mathbf{n}, \mathbf{z}} E_{\text{QPM}}(\mathbf{n}, \mathbf{z}, \tilde{\mathbf{z}}) = \sum_{k \in K} \min_{n_k, z_k} E_{\text{QPM}}^k(n_k, z_k) \quad \text{where} \quad (14)$$

$$E_{\text{QPM}}^k(n_k, z_k) = E_p^k(n_k, z_k) + \lambda_s E_s^k(n_k, \tilde{z}_k) + \sigma^{(i)}(\tilde{z}_k - z_k)^2 \quad (15)$$

$$E_p^k(n_k, z_k) = \frac{1}{|K|\mathcal{M}} \min_{|M_k|=\mathcal{M}} \sum_{m \in M_k} L_\delta(\Phi_m(n_k, z_k, \mathbf{c}))$$

$$E_s^k(n_k, \tilde{z}_k) = \frac{1}{|K||\mathcal{N}_k|} \sum_{j \in \mathcal{N}_k} (n_k^T(\tilde{\mathbf{x}}_k - \tilde{\mathbf{x}}_j))^2$$

$$\tilde{\mathbf{x}}_k = \tilde{z}_k(P_1^+ p_k - o_1) + o_1$$

The inputs to (15) have 3 degrees of freedom (DOFs) (2 for  $n_k$  and 1 for  $z_k$ ). Let us further assume that depth  $z_k$  is bounded and  $E_{\text{QPM}}^k$  is Lipschitz continuous, we may then resort to the DIRECT search approach [1] which guarantees global minimal solution despite non-convexity. Therefore  $E_{\text{QPM}}$  as a whole can be globally minimized in linear time complexity w.r.t.  $|K|$ . In practise, we used a randomized algorithm (PatchMatch) for searching optimal  $\{\mathbf{n}, \mathbf{z}\}$  for its computational efficiency.

### References

- [1] Robert Hooke and Terry A Jeeves. DIRECT search: Solution of numerical and statistical problems. *Journal of the ACM (JACM)*, 8(2):212–229, 1961. 3
- [2] Zhuo Hui, Kalyan Sunkavalli, Joon-Young Lee, Sunil Hadap, Jian Wang, and Aswin C Sankaranarayanan. Reflectance capture using univariate sampling of brdfs. In *Proceedings of*

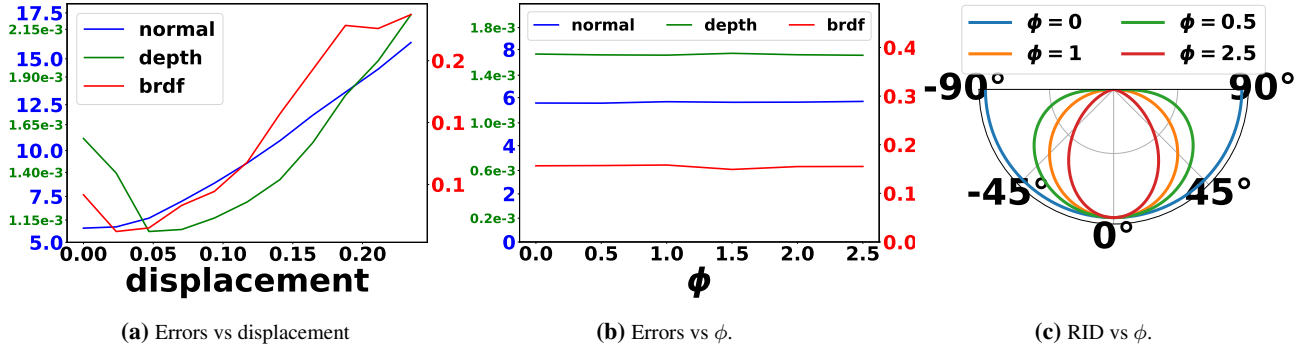

**Figure 3:** Normal mean angular and depth RMSE w.r.t. various degrees of light displacement and anisotropy.

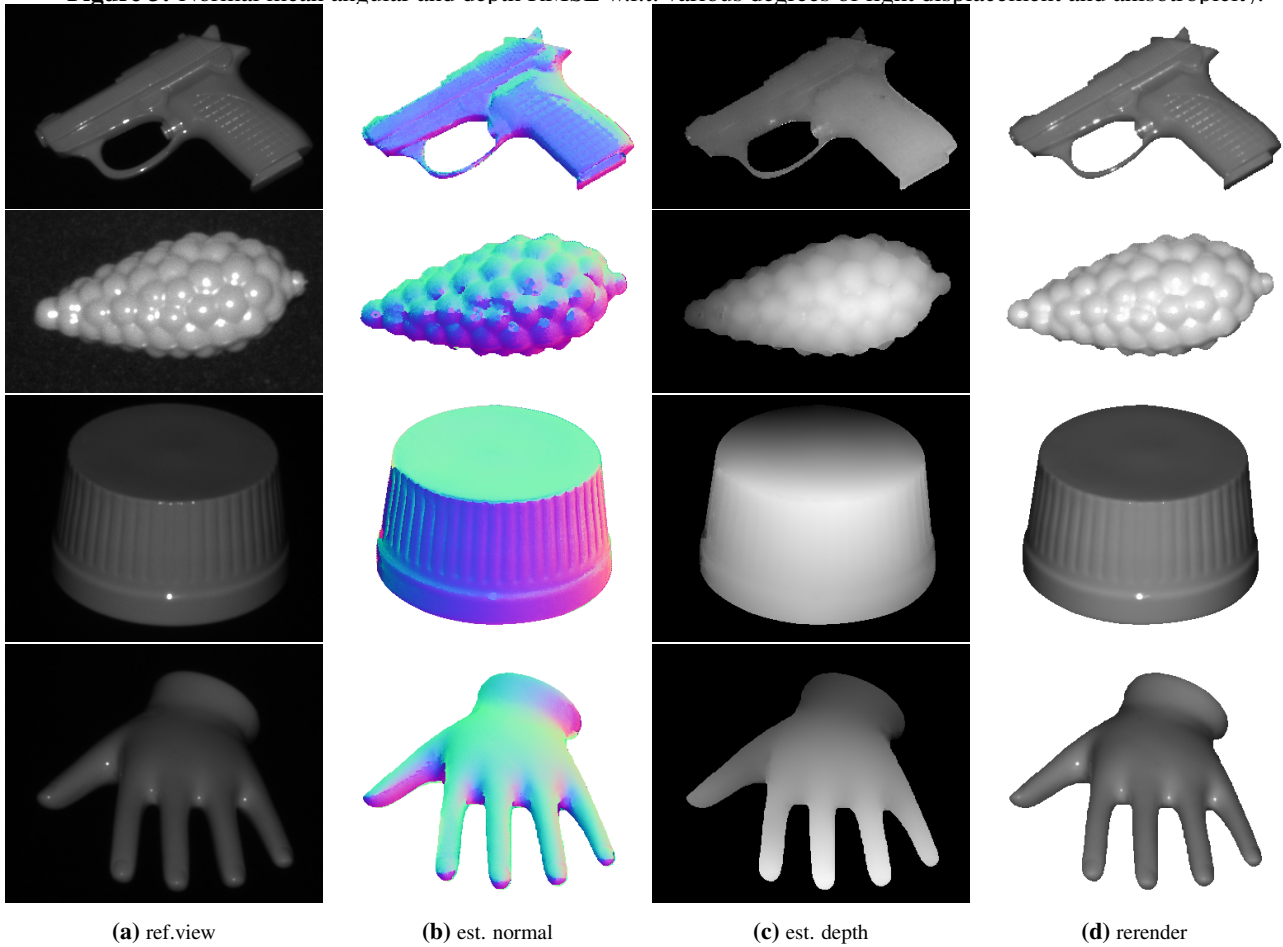

**Figure 4:** Recovered normal and depth maps for real-world objects.

the IEEE International Conference on Computer Vision, pages 5362–5370, 2017. 1

- [3] Wojciech Matusik, Hanspeter Pfister, Matt Brand, and Leonard McMillan. A data-driven reflectance model. *ACM Transactions on Graphics*, 22(3):759–769, July 2003. 1
- [4] Jannik Boll Nielsen, Henrik Wann Jensen, and Ravi Ramamoorthi. On optimal, minimal brdf sampling for reflectance acquisition. *ACM Transactions on Graphics (TOG)*,

34(6):186, 2015. 1, 3

- [5] Zexiang Xu, Jannik Boll Nielsen, Jiyang Yu, Henrik Wann Jensen, and Ravi Ramamoorthi. Minimal brdf sampling for two-shot near-field reflectance acquisition. *ACM Transactions on Graphics (TOG)*, 35(6):188, 2016. 1
